# Supplementary material for: On Delay-Optimal Scheduling in Queueing Systems with Replications
Source: arXiv:1603.07322 source file (2017-02-06)
Supplement: Supplementary file 1 [file appendices.tex]

% !TEX root = ./replication.tex
\ifreport
\appendices
\else
\appendix
\fi
\section{Proofs of Lemmas~1-3 and Corollaries 1-2} \label{app0}
\ifreport
\begin{proof}[Proof of Lemma \ref{lem1}]
\else
\begin{proof}[of Lemma \ref{lem1}]
\fi
First, fix the sequence of task completion times as $\bm{T}(\pi)=\bm{t}$ for all $\pi\in\Pi$. Because a job is completed at the time that the last task of the job is completed, each job completion time $C_i(\pi)$ must be equal to one element of $\bm{t}$. Using condition 2 and the sample-path optimality of the preemptive SRPT discipline \cite{Schrage68,Smith78}, one can obtain that for all $\pi\in\Pi$ and $\bm{t}\geq\bm{0}$
\begin{align}
[\bm{C}_{\uparrow} (P')|\bm{T}(P')=\bm{t}] \leq[\bm{C}_{\uparrow} (\pi)|\bm{T}(\pi)=\bm{t}],\nonumber
\end{align} 
where $\bm{C}_{\uparrow} (\pi)= (C_{(1)}(\pi),\ldots,$ $C_{(n)}(\pi))$ is the increasing time sequence of job completions. In addition, using the proof arguments in \cite{Schrage68,Smith78}, we can show that $[\bm{C}_{\uparrow} (P') | \bm{T}(P')=\bm{t}]$ is an increasing function of $\bm{t}$. This implies
\begin{align}\label{eq_order}
[\bm{C}_{\uparrow} (P')|\bm{T}(P')=\bm{t}] \leq[\bm{C}_{\uparrow} (\pi)|\bm{T}(\pi)=\bm{t}'],
\end{align} 
whenever $\bm{0}\leq\bm{t}\leq \bm{t}'$. On the other hand, condition 1 tells us that for all $\pi\in\Pi$ and $\mathcal{I}$
\begin{align}\label{eq_order_}
[\bm{T}(P')|\mathcal{I}] \leq_{\text{st}}[\bm{T}(\pi)|\mathcal{I}].
\end{align} 
%Therefore, 
%\begin{align}
%[{D}_{\text{avg}}(\bm{C}_{} (P))|\mathcal{I}] \leq_{\text{st}}[{D}_{\text{avg}}(\bm{C}_{} (\pi))|\mathcal{I}].\nonumber
%\end{align} 
According to Theorem 6.B.3 and Theorem 6.B.16(c) of \cite{StochasticOrderBook}, we can obtain from  \eqref{eq_order} and \eqref{eq_order_} that
\begin{align}\label{eq_order_1}
[\bm{C}_{\uparrow} (P')|\mathcal{I}] \leq_{\text{st}}[\bm{C}_{\uparrow} (\pi)|\mathcal{I}].
\end{align} 
Combining this and condition 3, we can get
\begin{align}
[\bm{U}_{\uparrow} (P)|\mathcal{I}] \leq_{\text{st}}[\bm{C}_{\uparrow} (\pi)|\mathcal{I}].\nonumber
\end{align} 
Since ${D}_{\text{avg}}\in \mathcal{D}_{\text{sym}}$ is symmetric and increasing, we can obtain that for all $\pi\in\Pi$ and $\mathcal{I}$
\begin{align}
&[{D}_{\text{avg}}(\bm{U} (P))|\mathcal{I}]=[{D}_{\text{avg}}(\bm{U}_{\uparrow} (P))|\mathcal{I}] \nonumber\\
\leq_{\text{st}}&[{D}_{\text{avg}}(\bm{C}_{\uparrow} (\pi))|\mathcal{I}] = [{D}_{\text{avg}}(\bm{C} (\pi))|\mathcal{I}],\nonumber
\end{align} 
where the inequality follows from Theorem 6.B.16(a) of \cite{StochasticOrderBook}. By this, \eqref{eq_lem1_1} is proven.

If condition 3 is replaced by $P'=P$, then \eqref{eq_lem1_2} follows from \eqref{eq_order_1} and Theorem 6.B.16(a) of \cite{StochasticOrderBook}. This completes the proof.
\end{proof}
\ifreport
\begin{proof}[Proof of Corollary \ref{coro1}]
\else
\begin{proof}[of Corollary \ref{coro1}]
\fi
Corollary \ref{coro1} is proven by replacing ${D}_{\text{avg}}$ in the proof of Lemma \ref{lem1} with any $f\in\mathcal{D}_{\text{sym}}$.
\end{proof}

\ifreport
\begin{proof}[Proof of Lemma \ref{lem2}]
\else
\begin{proof}[of Lemma \ref{lem2}]
\fi

First, fix the sequence of task completion times such that $\bm{T}(P')=\bm{T}(\pi)=\bm{t}$ for all $\pi\in\Pi$. Using condition 2 and the sample-path optimality of the preemptive earliest due date (EDD) discipline \cite{Jackson55}, one can obtain that for all $\pi\in\Pi$ and $\bm{t}\geq\bm{0}$
\begin{align}
[L_{\max}(\bm{C}(P'))|\bm{T}(P')=\bm{t}] \leq[L_{\max}(\bm{C}(\pi))|\bm{T}(\pi)=\bm{t}].\nonumber
\end{align} 
In addition, one can show that $[L_{\max}(\bm{C}(P')) | \bm{T}(P')=\bm{t}]$ is increasing in $\bm{t}$. Hence,
\begin{align}\label{eq_lem2_order1}
[L_{\max}(\bm{C}(P'))|\bm{T}(P')=\bm{t}] \leq[L_{\max}(\bm{C}(\pi))|\bm{T}(\pi)=\bm{t}'],
\end{align} 
whenever $\bm{0}\leq\bm{t}\leq \bm{t}'$. On the other hand, condition 1 tells us that for all $\pi\in\Pi$ and $\mathcal{I}$
\begin{align}\label{eq_lem2_order2}
[\bm{T}(P')|\mathcal{I}] \leq_{\text{st}}[\bm{T}(\pi)|\mathcal{I}].
\end{align} 
Using \eqref{eq_lem2_order1}, \eqref{eq_lem2_order2}, Theorem 6.B.3, and Theorem 6.B.16(c) of \cite{StochasticOrderBook}, yields that for all $\pi\in\Pi$ and $\mathcal{I}$
\begin{align}\label{eq_lem2_order3}
[L_{\max}(\bm{C}(P'))|\mathcal{I}] \leq_{\text{st}}[L_{\max}(\bm{C}(\pi))|\mathcal{I}].
\end{align} 
Using condition 3, the fact that $L_{\max}$ is increasing, and Theorem 6.B.16(a) of \cite{StochasticOrderBook}, we can obtain 
\begin{align}\label{eq_lem2_order4}
[L_{\max}(\bm{U}(P))|\mathcal{I}]\leq_{\text{st}} [L_{\max}(\bm{C}(P'))|\mathcal{I}].
\end{align} 
Combining \eqref{eq_lem2_order3} and \eqref{eq_lem2_order4}, \eqref{eq_lem2_1} follows. If condition 3 is replaced by $P'=P$, then 
\eqref{eq_lem2_2} follows from \eqref{eq_lem2_order3}. This completes the proof.
\end{proof}
\ifreport
\begin{proof}[Proof of Corollary \ref{coro2}]
\else
\begin{proof}[of Corollary \ref{coro2}]
\fi
We need the rearrangement partial ordering $\leq^{\text{a}}$ defined in \cite[Sec. 6.F]{Marshall2011}: Consider two $n$-vector $\bm{x}$ and $\bm{y}$, $\bm{x}$ is said to \emph{immediately precede} $\bm{y}$ by one pairwise interchange, denote $\bm{x}<^{\text{p}}\bm{y}$, if for some index $i$, $1\leq i\leq n-1$,
\begin{align}
y_i<y_{i+1}, ~x_i= y_{i+1}, ~x_{i+1}=y_i, ~x_l= y_l,~l\neq i,i+1.\nonumber
\end{align}
Let $\leq^{\text{b}}$ denote the ordering of successive interchanges, such that $\bm{x}\leq^{\text{b}}\bm{y}$ if $\bm{x}=\bm{y}$ or if there exists a finite chain $\bm{z}^1,\ldots,\bm{z}^k$ of permutations such that
\begin{align}
\bm{x}<^{\text{p}}\bm{z}^1<^{\text{p}}\ldots<^{\text{p}}\bm{z}^k<^{\text{p}}\bm{y}.\nonumber
\end{align}
Suppose that $\bm{x}$ is a permutation of $\bm{u}$ and $\bm{y}$ is a permutation of $\bm{v}$ such that $\bm{x}_{\uparrow}=\bm{u}_{\uparrow}$ and $\bm{y}_{\uparrow}=\bm{v}_{\uparrow}$. Then, $(\bm{x},\bm{y})\leq^{\text{a}} (\bm{u},\bm{v})$ if there exists permutation matrices $W$ and $U$ such that
\begin{align}
\bm{x}W = \bm{u} U=\bm{x}_{\uparrow},~~~\text{and}~~ \bm{y} W \leq^{\text{b}} \bm{v} U.\nonumber
\end{align}
Hence, one can obtain
\begin{align}
(\bm{x}_{\uparrow},\bm{y}_{\downarrow})\leq^{\text{a}}(\bm{x},\bm{y})\leq^{\text{a}}(\bm{x}_{\uparrow},\bm{y}_{\uparrow}).\nonumber
\end{align}
The following rearrangement inequality is an immediate consequence of Theorem F.14 in Chapter 6 of \cite{Marshall2011}:
\begin{lemma}\label{lem_coro_2}
If \emph{$(\bm{x},\bm{y})\geq^{\text{a}} (\bm{u},\bm{v})$}, then
\begin{align}
\bm{x}-\bm{y}\prec \bm{u}-\bm{v}.\nonumber
\end{align}
\end{lemma}

Now, we are ready to prove Corollary \ref{coro2}. As before, we first fix the sequence of task completion times such that $\bm{T}(P')=\bm{T}(\pi)=\bm{t}$ for all $\pi\in\Pi$. Since $k_1=\ldots=k_n=1$, $\bm{C}(P')$ and $\bm{C}(\pi)$ are permutations of $\bm{t}$. According to condition 2 of Lemma \ref{lem2}, each completed job of policy $P'$ has the smallest due time $d_i$ among all unfinished jobs in the queue. Hence,
\begin{align}
[(\bm{C}(P'), \bm{d}) |\bm{T}(P')=\bm{t}] \geq^{\text{a}} [(\bm{C}(\pi), \bm{d}) |\bm{T}(\pi)=\bm{t}].\nonumber
\end{align}
Then, Lemma \ref{lem_coro_2} tells us that for all $\pi\in\Pi$
\begin{align}\label{eq_coro2_4}
&[\bm{L} (P') |\bm{T}(P')=\bm{t}]\nonumber\\
=&[\bm{C}(P') - \bm{d}|\bm{T}(P')=\bm{t}]\nonumber\\
\prec& [\bm{C}(\pi) - \bm{d}|\bm{T}(\pi)=\bm{t}] \nonumber\\
=&[\bm{L}(\pi)|\bm{T}(\pi)=\bm{t}]. 
\end{align} 
%it is easy to show that $t_{i}\leq {C}_{(i)}(\pi)$ for all $i=1,2,\ldots, n$ and $\pi\in\Pi$. Using condition 2 of Lemma \ref{lem2}, we can obtain that for all $\pi\in\Pi$
%\begin{align}\label{eq_coro2_1}
%[\bm{C}_{\uparrow}(P')|\bm{T}(P')=\bm{t}] = (t_1,t_{2},\ldots,t_{n}) \leq [\bm{C}_{\uparrow}(\pi)|\bm{T}(\pi)=\bm{t}].
%\end{align} 
%On the other hand, the rearrangement inequality \cite[Theorem F.14 of Sec. 6]{Marshall2011} implies that for all $\pi\in\Pi$
%\begin{align}\label{eq_coro2_2}
%\bm{C}_{\uparrow}(\pi) - \bm{d}_{\uparrow} \prec \bm{C}(\pi) - \bm{d}.
%\end{align} 
%In addition, condition 2 of Lemma \ref{lem2} tells us that the jobs are completed in the increasing order of $\bm{d}$. Hence, the job completed at time $C_{(i)}(P')$ has a due time $d_{(i)}$ for all $i=1,\ldots,n$. This implies
%\begin{align}\label{eq_coro2_3}
%\bm{L}_{\uparrow} (P')= \bm{C}_{\uparrow}(P') - \bm{d}_{\uparrow}.
%\end{align} 
%Combining \eqref{eq_coro2_1}-\eqref{eq_coro2_3}, yields for all $\pi\in\Pi$
%\begin{align}\label{eq_coro2_4}
%&[\bm{L}_{\uparrow} (P') |\bm{T}(P')=\bm{t}]\nonumber\\
%=&[\bm{C}_{\uparrow}(P') - \bm{d}_{\uparrow}|\bm{T}(P')=\bm{t}]\nonumber\\
%\leq&[\bm{C}_{\uparrow}(\pi)- \bm{d}_{\uparrow}|\bm{T}(\pi)=\bm{t}]\nonumber\\
%\prec& [\bm{C}(\pi) - \bm{d}|\bm{T}(\pi)=\bm{t}] \nonumber\\
%=&[\bm{L}(\pi)|\bm{T}(\pi)=\bm{t}]. 
%\end{align} 
For any $f\in\mathcal{D}_{\text{Sc}}$, define $g(\bm{x})=f(\bm{x}+\bm{d})$. Then, $g$ is Schur convex. For $\pi\in\Pi$, we can obtain
\begin{align}
&[f(\bm{C} (P')) |\bm{T}(P')=\bm{t}]\nonumber\\
=&[g(\bm{L} (P') ) |\bm{T}(P')=\bm{t}]\nonumber\\
\leq&[g(\bm{L} (\pi)) |\bm{T}(\pi)=\bm{t}]\nonumber\\
=&[f(\bm{C} (\pi)) |\bm{T}(\pi)=\bm{t}],\nonumber
\end{align}
where the inequality is due to \eqref{eq_coro2_4} and the definition of Schur convex functions. The remaining proof is the same as \eqref{eq_lem2_order1}-\eqref{eq_lem2_order4}, where we will need to use the fact that $f$ is increasing.
\end{proof}

\ifreport
\begin{proof}[Proof of Lemma \ref{lem3}]
\else
\begin{proof}[of Lemma \ref{lem3}]
\fi
Using \eqref{eq_lem3_1} and $\bm{U}(\pi)\leq\bm{C}(\pi)$, we can obtain $[\bm{U}(P)|\mathcal{I}] \leq_{\text{st}} [\bm{C}(\pi)|\mathcal{I}]$ for all $\pi\in\Pi_{PL}$. By this, Theorem 6.B.4.(a) of \cite{StochasticOrderBook}, and the fact that $f$ is increasing, \eqref{eq_lem3_2} follows. This completes the proof.
\end{proof}
