# Supplementary material for: On Delay-Optimal Scheduling in Queueing Systems with Replications
Source: arXiv:1603.07322 source file (2017-02-06)
Supplement: Supplementary file 4 [file appendices_5.tex]

% !TEX root = ./replication.tex

\section{Proofs of Thoerem~4 and Corollary 6} \label{app4}
\subsection{Proof of Thoerem~\ref{thm4}} \label{sec_app_4_1}
We prove Thoerem~\ref{thm4} by using Lemma \ref{lem2}, where the policy space $\Pi$ is replaced by $\Pi_{\text{non-prmp}}$ because preemption is not allowed. The proof steps are as follows:

{\bf Construction of Policy $P'$:}
We construct an {infeasible} policy $P'$. Similar with policy EDD-R, when all servers are idle in policy $P'$, a task from the job with the earliest due time is replicated on all $m$ servers. When a copy of this task is completed, the remaining $m-1$ replicated copies of this task are cancelled. The difference between policy EDD-R and policy $P'$ is that \emph{the completed tasks of policy $P'$ are relabelled such that each completed task is from the job with the earliest due time}. (This relabeling operation might be infeasible in the following scenario: If a job with an earlier due time arrives, the servers cannot be reassigned to this incoming job because preemption is not allowed. However, the next completed task is relabelled to be from this incoming job which has the earliest due time.) By this, policy $P'$ is constructed.

Next, we prove the conditions of Lemma \ref{lem2} one by one.

\textbf{Condition 1:} \emph{Policy $P'$ is more {work-efficient} than any policy $\pi\in\Pi_{\text{non-prmp}}$}. Condition 1 can be proven by using the same proof arguments in Appendix \ref{sec_app_thm2_1}.

\textbf{Condition 2:} \emph{Each completed task of policy $P'$ belongs to the job with the earliest due time}. Condition 2 directly follows from the construction of policy $P'$.

\textbf{Condition 3:} \emph{It holds that} 
\begin{align}\label{eq_condition3_thm4}
[\bm{U}_{}(\text{EDD-R})|\mathcal{I}] \leq_{\text{st}} [\bm{C}_{}(P')|\mathcal{I}].
\end{align}

We prove condition 3 by using the \emph{sample-path ordering} technique. The system state $\bm{\xi}$ of policy $P'$ is the same as that in \emph{Definition \ref{def_state_P_thm3}}. The system state $(\bm{\gamma},\bm{\zeta})$ of policy EDD-R is the same as that in \emph{Definition \ref{def_state_thm3}}. 
In policy EDD-R, all servers are simultaneously assigned to process $m$ replicated copies of the same task. Hence, $\bm{\zeta}$ satisfies
\begin{align}
\zeta_i\in\{0,1\},~\sum_{i=1}^n \zeta_i\leq1.
\end{align}
We can prove that Lemmas \ref{lemG4_thm3}-\ref{lem_non_prmp2_thm3} hold for policy EDD-R. 
Using Lemma \ref{lemG4_thm3}, condition 3 can be proven by using the same proof arguments in Appendix \ref{sec_app_3_1}, where policy EDD-NR should be replaced by policy EDD-R.

After establishing conditions 1-3 of Lemma \ref{lem2} for policy EDD-R,  we can use Lemma \ref{lem2} to prove Theorem \ref{thm4}. This completes the proof.

\subsection{Proof of Corollary~\ref{coro4_2}}  
If $d_1\leq\ldots\leq d_n$, then each completed task of policy EDD-R belongs to the job with the earliest due time. Therefore, policy EDD-R is identical with policy $P'$ constructed in Appendix \ref{sec_app_4_1}. Then, Corollary \ref{coro4_2} follows from Lemma \ref{lem2}. 

\subsection{Proof of Corollary~\ref{coro4_1}} \label{sec_app_4_2} 
Because conditions 1-3 of Lemma \ref{lem2} have been established in Appendix \ref{sec_app_4_1},  Corollary~\ref{coro4_1} directly follows from Corollary \ref{coro2}.
