# Supplementary material for: On Delay-Optimal Scheduling in Queueing Systems with Replications
Source: arXiv:1603.07322 source file (2017-02-06)
Supplement: Supplementary file 5 [file appendices_6.tex]

% !TEX root = ./replication.tex

\section{Proof of Thoerem~5} \label{app5}

\subsection{Proof of \eqref{eq_delaygap1_thm5} in Thoerem~5}
We prove \eqref{eq_delaygap1_thm5} in Thoerem~\ref{thm5} by using Lemma \ref{lem3}. In particular, we will use the \emph{sample-path ordering} technique to prove condition \eqref{eq_lem3_1} of Lemma \ref{lem3}.
We first define the system states of policy PL-NR and any policy $\pi\in\Pi_{PL}$, where $PL=(p_1,\ldots,p_n)$ denote a static priority list.

\begin{definition}\label{def_state_P_thm5}
The system state of policy $\pi\in\Pi_{PL}$ is specified by a pair of $n$-dimensional vectors $\bm{\xi}=(\xi_1,\ldots,\xi_n)$ and $\bm{\kappa}=(\kappa_1,\ldots,\kappa_n)$ with non-negative components. At any time, if job $i$ exists in the system, $\xi_i$ is the number of remaining tasks of job $i$ and $\kappa_i$ out of these $\xi_i$ tasks are under service on some servers; if job $i$ has not arrived at the system or has departed from the system, $\xi_i=\kappa_i=0$. Hence, 
\begin{align}%\label{eq_def_state_P_thm5}
\kappa_i  \leq \xi_i \leq k_{i},~\sum_{i=1}^n \kappa_i \leq m. \nonumber
\end{align}
\end{definition}

\begin{definition}\label{def_state_thm5}
The system state of policy PL-NR is specified by a pair of $n$-dimensional vectors $\bm{\gamma}=(\gamma_1,\ldots,\gamma_n)$ and $\bm{\zeta}=(\zeta_1,\ldots,\zeta_n)$ with non-negative components. 
At any time, if job $i$ exists in the system, then $\gamma_i$ is the number of remaining tasks of job $i$ and $\zeta_i$ out of these $\gamma_i$ tasks are under service on some servers; if job $i$ has not arrived at the system or has departed from the system, then $\gamma_i=\zeta_i=0$.
Hence, 
\begin{align}%\label{eq_def_state_thm5}
\zeta_i  \leq \gamma_i \leq k_{i},~\sum_{i=1}^n \zeta_i \leq m. \nonumber
\end{align}
\end{definition}

Let $\{\bm{\xi}(t),\bm{\kappa}(t),t\geq0\}$ be the state process of policy $\pi$, and $\{\bm{\gamma}(t),\bm{\zeta}(t),t\geq0\}$ be the state process of PL-NR, which are assumed to be right-continuous. 
The sample-path ordering result is stated in the following lemma:

\begin{lemma}\label{lemG4_thm5}
Suppose that $\bm{\xi}(0^-)=\bm{\kappa}(0^-)=\bm{\gamma}(0^-)=\bm{\zeta}(0^-)=\bm{0}$ and the job parameters $\mathcal{I}$ are given. For any sample path of policy PL-NR, there exists a sample path of policy $\pi$ with the same probability density such that
\begin{eqnarray}\label{eq_lemG4_thm5}
\sum_{i:p_i\geq p} [\gamma_i(t) - \zeta_i(t)]\leq \sum_{i:p_i\geq p} [\xi_i(t)-\kappa_i(t)], 
\end{eqnarray}
holds for all $t\geq0$ and $p = 1,2,\ldots,n$.
\end{lemma}

The following two lemmas are needed to prove Lemma \ref{lemG4_thm5}:

\begin{lemma}\label{lem_non_prmp1_thm5}
Suppose that, under policy PL-NR, $\{\bm{\gamma}',\bm{\zeta}'\}$ is obtained by completing a task on one server in the system whose state is $\{\bm{\gamma},\bm{\zeta}\}$. Further, suppose that, under policy $\pi$, $\{\bm{\xi}',\bm{\kappa}'\}$ is obtained by completing a task on one server in the system whose state is $\{\bm{\xi},\bm{\kappa}\}$. If
\begin{eqnarray}
\sum_{i:p_i\geq p} [\gamma_i - \zeta_i]\leq \sum_{i:p_i\geq p} [\xi_i-\kappa_i], ~\forall~p = 1,2,\ldots,n,\nonumber
\end{eqnarray}
then
\begin{eqnarray}\label{eq_non_prmp_40_thm5}
\sum_{i:p_i\geq p} [\gamma_i'- \zeta_i']\leq \sum_{i:p_i\geq p} [\xi_i'-\kappa_i'], ~\forall~p = 1,2,\ldots,n.\end{eqnarray}
\end{lemma}

\begin{proof}
If $\sum_{i:p_i\geq p} [\gamma_i' - \zeta_i']=0$, then the inequality \eqref{eq_non_prmp_40_thm5} follows naturally. 
If $\sum_{i:p_i\geq p} [\gamma_i' - \zeta_i']>0$, then there exist some tasks that have not been assigned to any server. 
In both policy PL-NR and policy $\pi$, a server that has just completed a task will be allocated to process an unassigned task from the job with the highest priority among all jobs in the queue. Hence,
$\sum_{i:p_i\geq p} [\gamma_i' - \zeta_i']=\sum_{i:p_i\geq p} [\gamma_i - \zeta_i] - 1 \leq \sum_{i:p_i\geq p} [\xi_i-\kappa_i] -1 \leq \sum_{i:p_i\geq p} [\xi_i'-\kappa_i']$.
\end{proof}

\begin{lemma}\label{lem_non_prmp2_thm5}
Suppose that, under policy PL-NR, $\{\bm{\gamma}',\bm{\zeta}'\}$ is obtained by adding a job with $b$ tasks and priority $d$ to the system whose state is $\{\bm{\gamma},\bm{\zeta}\}$. Further, suppose that, under policy $\pi$, $\{\bm{\xi}',\bm{\kappa}'\}$ is obtained by adding a job with $b$ tasks and priority $d$ to the system whose state is $\{\bm{\xi},\bm{\kappa}\}$.
If
\begin{eqnarray}
\sum_{i:p_i\geq p} [\gamma_i- \zeta_i]\leq \sum_{i:p_i\geq p} [\xi_i-\kappa_i], ~\forall~p = 1,2,\ldots,n,\nonumber
\end{eqnarray}
then
\begin{eqnarray}
\sum_{i:p_i\geq p} [\gamma_i' - \zeta_i']\leq \sum_{i:p_i\geq p} [\xi_i'-\kappa_i'], ~\forall~p = 1,2,\ldots,n.\nonumber\end{eqnarray}
\end{lemma}

\begin{proof}
If $d\geq p$, then
$\sum_{i:p_i\geq p} [\gamma_i' - \zeta_i']\leq \sum_{i:p_i\geq p} [\gamma_i - \zeta_i] + b\leq \sum_{i:p_i\geq p} [\xi_i-\kappa_i]+b \leq \sum_{i:p_i\geq p} [\xi_i'-\kappa_i']$.

If $d<p$, then
$\sum_{i:p_i\geq p} [\gamma_i' - \zeta_i']\leq \sum_{i:p_i\geq p} [\gamma_i - \zeta_i] \leq \sum_{i:p_i\geq p} [\xi_i-\kappa_i] \leq \sum_{i:p_i\geq p} [\xi_i'-\kappa_i']$.
\end{proof}

Now we are ready to prove Lemma \ref{lemG4_thm5}.
\ifreport
\begin{proof}[Proof of Lemma \ref{lemG4_thm5}]
\else
\begin{proof}[of Lemma \ref{lemG4_thm5}]
\fi
Consider any period $[\tau,\nu)$ of policy PL-NR, during which there are at least $m$ tasks such that all $m$ servers are busy. We prove \eqref{eq_lemG4_thm5} for $t\in[\tau,\nu)$ by considering two cases:

\emph{Case 1: At time $t=\tau$, policy PL-NR has $m$ tasks and the service of these tasks has just started.} Consider the system states of both policies at time $\tau$. The system state of policy PL-NR satisfies 
\begin{align}\label{proof_lemG4_1_thm5}
\sum_{i=1}^n \gamma_i(\tau)= m, ~\bm{\gamma}(\tau)=\bm{\zeta}(\tau).
\end{align}
In policy $P'$, there is no task in the system at time $\tau^-$ such that 
\begin{align}\label{proof_lemG4_5_thm5}
\bm{\xi}(\tau^-)=\bm{0}. 
\end{align}
Consider the evolutions of both policies during $[\tau,\nu)$. 
In policy $P'$, all servers are busy if there is at least one task. On the other hand, in policy EDD-NR, there is no task replication and all servers are busy if there are no less than $m$ tasks. 
By \eqref{proof_lemG4_1_thm5} and \eqref{proof_lemG4_5_thm5}, it holds that for $t=\tau$
\begin{align}\label{proof_lemG4_4_thm5}
\sum_{i=1}^n \gamma_i(t)= \sum_{i=1}^n\xi_i(t) +m\geq m+1.
\end{align}
Therefore, the servers are all busy in policies $P'$ and policy EDD-NR at time $\tau$. By induction over time, we can show that for any sample path of policy $P'$, there is a sample path of policy EDD-NR with the same probability density such that \eqref{proof_lemG4_4_thm5} holds for all $t\in[\tau,\nu)$ and the task arrival times and task completion times of the two policies are exactly the same  during $[\tau,\nu)$. Using Lemma \ref{lem_non_prmp1_thm5}, Lemma \ref{lem_non_prmp2_thm5}, and the initial states at time $\tau^-$, we can prove that \eqref{eq_lemG4_thm5} holds for all $t\in[\tau,\nu)$ on these two sample paths.

\emph{Case 2: At time $t=\tau^-$, policy EDD-NR has less than $m$ tasks or the service of these tasks started before time $\tau^-$}. In both \emph{Case 1} and \emph{Case 2}, the sample path evolutions of policy $P'$ are the same. On the other hand, in policy EDD-NR, the tasks are completed earlier in \emph{Case 2} than in \emph{Case 1}. Therefore, \eqref{eq_lemG4_thm5}  also holds in \emph{Case 2} for $t\in[\tau,\nu)$.

%Note that the case that policy EDD-NR has more than $m$ tasks at time $\tau^-$ will not happen. This will be clear 
Let $[\tau_1,\nu_1)$ be the next busy period of policy $P'$ with $\nu<\tau_1$. Then, $[\nu,\tau_1)$ is an idle period of policy $P'$. We now prove \eqref{eq_lemG4_thm5} during the idle period $[\nu,\tau_1)$. 
Because all servers are idle during $[\nu,\tau_1)$ in policy $P'$, it follows that 
\begin{align}\label{proof_lemG4_2_thm5}
\bm{\xi}(t)=\bm{0},~t\in[\nu,\tau_1).
\end{align}
Hence, there is no task arrival during $[\nu,\tau_1)$; otherwise, \eqref{proof_lemG4_2_thm5} cannot be true.
On the other hand, at time $\nu$ there are no more than $m$ tasks in policy EDD-NR such that 
\begin{align}
\bm{\gamma}(\nu)=\bm{\zeta}(\nu).\nonumber
\end{align}
Because there is no task arrival during $[\nu,\tau_1)$, policy EDD-NR satisfies
\begin{align}\label{proof_lemG4_3_thm5}
\bm{\gamma}(t)=\bm{\zeta}(t),~t\in[\nu,\tau_1).
\end{align}
By \eqref{proof_lemG4_2_thm5} and \eqref{proof_lemG4_3_thm5}, \eqref{eq_lemG4_thm5} holds during $[\nu,\tau_1)$.
Further, from \eqref{proof_lemG4_3_thm5}, we can obtain
\begin{align}
\sum_{i=1}^n \gamma_i(\tau_1^-)=\sum_{i=1}^n \zeta_i(\tau_1^-)\leq m,
\end{align}
such that there are no more than $m$ tasks at time $t=\tau_1^-$ in policy EDD-NR. Hence, either \emph{Case 1} or \emph{Case 2} is satisfied at time $t=\tau_1^-$. Then, we can use the above arguments to prove that  \eqref{eq_lemG4_thm5} holds during the next busy period $[\tau_1,\nu_1)$ of policy $P'$.

Finally, by taking an induction over the busy and idle periods of policy $P'$,  Lemma \ref{lemG4_thm5} is proven.
\end{proof}

After establishing conditions 1-3 of Lemma \ref{lem2} for policy EDD-R,  we can use Lemma \ref{lem2} to prove Theorem \ref{thm4}. This completes the proof.

\subsection{Proof of Corollary~\ref{coro4_2}}  
If $d_1\leq\ldots\leq d_n$, then each completed task of policy EDD-R belongs to the job with the earliest due time. Therefore, policy EDD-R is identical with policy $\pi$ constructed in Appendix \ref{sec_app_4_1}. Then, Corollary \ref{coro4_2} follows from Lemma \ref{lem2}. 

\subsection{Proof of Corollary~\ref{coro4_1}} \label{sec_app_4_2} 
Because conditions 1-3 of Lemma \ref{lem2} have been established in Appendix \ref{sec_app_4_1},  Corollary~\ref{coro4_1} directly follows from Corollary \ref{coro2}.
